# Supplementary material for: Local work function on Graphene Nanoribbons and on the Au(111) herringbone reconstruction
Source: arXiv:2203.06945 source file (2022-03-14)
Supplement: Supplementary file 1 [file Rothhardt_KPFM-GNR-SI.pdf]

# Supporting Information: Local work function on Graphene Nanoribbons and on the Au(111) herringbone reconstruction

*D. Rothhardt, A. Kimouche, T. Klamroth, R. Hoffmann-Vogel*

## 1 Methods

Experimental methods: The experiments were conducted in an Omicron variable temperature VT-SFM system under a base pressure of about $2 \cdot 10^{-10}$ mbar. We use commercially available Au on mica substrates (Georg Albert PVD, Germany) and clean them by Ar ion sputtering-annealing cycles. The cleanliness of the samples was checked by SFM measurments. Then $10-10-dibromo-9-9$ *bianthryl* (DBBA) molecules were deposited by thermal evaporation (Kentax evaporator) onto the hot ($T_{\text{sample}} = 470$ K) sample surface. The deposition rate was kept constant using a quartz crystal mircobalance. After deposition the sample was kept at 470 K for 10 min followed by annealing up to 670 K for 10 min. The sample was introduced into our SFM attached to the same vacuum chamber which was cooled down to 115 K using liquid nitrogen. Nanosensors tips with a resonance frequency of about 158 kHz and a longitudinal force constant of 45 N/m were used for imaging in the dynamic frequency modulation (FM) mode operated by a Nanonis electronics. The tips were cleaned by sputtering and annealing up to 340 K prior to measurement.

Kelvin probe force microscopy imaging was performed in parallel to topographic imaging using an AC excitation voltage of $V_{AC} = 600$ mV and $f_{AC} = 166$ Hz. AC and DC biases were applied to the sample. The polarity of the KPFM results were cross-checked on well-known surfaces, i.e. Si(111) and Pb on Si(111) to ensure that they are compatible with previous results [1, 2].

Theoretical methods: All calculations were done using the Vienna Ab initio Simulation Package[3, 4] (vasp-5.4.4) using the PBE functional[5] and a projector-augmented plane-wave basis (PAW)[6, 7]. Dispersion forces are included using Grimmes D3 method[8] with Becke-Jonson damping[9] (`IVDW=12`). Further, we include non-spherical contributions from the gradient corrections inside the PAW spheres (`LASPH = .TRUE.`). For all slab calculations the lowest gold layer was fixed using the optimized bulk lattice constant ($a_{\text{Au}} = 2.897367$ Å). The initial positions for the geometry optimizations are chosen according to the structure reported in Ref. [10].

Convergence test were made for a small orthorombic unit cell, i.e., $a = 3 \times a_{\text{Au}}$, $b = 3\sqrt{3} \times a_{\text{Au}}$ and $c$ set to a value, that about 15 Å of vacuum is in between the slabs. Here, $c$ is pointing in the surface normal direction ($z$), $a$ is the direction of the GNR ($x$) and $b$ provides about 5.8 Å spacing

between two GNRs (smallest distance between two hydrogen cores). We used up to seven Gold layers, cutoff energies up to 700 eV and $k$-point grids up to $7 \times 7 \times 1$. We found the optimized geometries and the LCPD maps just above the surface, i.e. for $s = 0$, to be converged for three gold layers with a cutoff energy of 400 eV and a $4 \times 4 \times 1$ $k$-point grid.

This parameters are also used for the large orthorombic unit cell ($a = 3 \times a_{\mathrm{Au}}$, $b = 4\sqrt{3} \times a_{\mathrm{Au}}$, $c = 50$ Å), which was used for the calculations of the LCPD maps in Figure 3 of the main text and in this supporting information, Fig. 1. Here, the vacuum thickness is increased to $\approx 42$ Å and the spacing between two GNRs to 10.8 Å. For the optimized geometry the Hartree potential, $V_{\mathrm{eff}}(\underline{r})$, (`LVHAR=.TRUE.`) was calculated using monopole/dipole and quadrupole corrections to the total energy in the surface normal direction (`IDIPOL=3` and `LDIPOL=.TRUE.`).

Fig. 1 shows further details about the performed calculations. **a** shows the large orthorombic unit cell used in the calculations, where all atomic positions are optimized, expect the ones of the lowest gold layer. **b** shows a $4 \times 1$ surface unit cell, which corresponds to the LCPD maps shown in **d** and Fig. 3 of the publication. Also indicated in **b** are the horizontal planes used to determine the LCPD maps for $s = 0$Å (red), $s = 2$Å (yellow) and $s = 4$Å (blue). A top view of the same cell as in **b** is shown in **c**.

# References


[1] C. Pérez León, H. Drees, S. M. Wippermann, M. Marz, and R. Hoffmann-Vogel, J. Phys. Chem. Lett. **7**, 426 (2016)

[2] Th. Späth, M. Popp, C. Pérez León, M. Marz and R. Hoffmann-Vogel, Nanoscale **9**, 7868 (2017)

[3] G. Kresse and J. Furthmüller, Comput. Mater. Sci. **6**, 15 (1996)

[4] G. Kresse and J. Furthmüller, Phys. Rev. B **54**, 11169 (1996)

[5] J. P. Perdew, K. Burke, and M. Ernzerhof, Phys. Rev. Lett. **77**, 3865 (1996)

[6] P. E. Blöchl, Phys. Rev. B **50**, 17953 (1994)

[7] G. Kresse and D. Joubert, Phys. Rev. B **59**, 1758 (1999)

[8] S. Grimme, J. Antony, S. Ehrlich, and S. Krieg, J. Chem. Phys. **132**, 154104 (2010)

[9] S. Grimme, S. Ehrlich, and L. Goerigk, J. Comp. Chem. **32**, 1456 (2011)

[10] L. Liang and V. Meunier, Phys. Rev. B **86**, 195404 (2012)

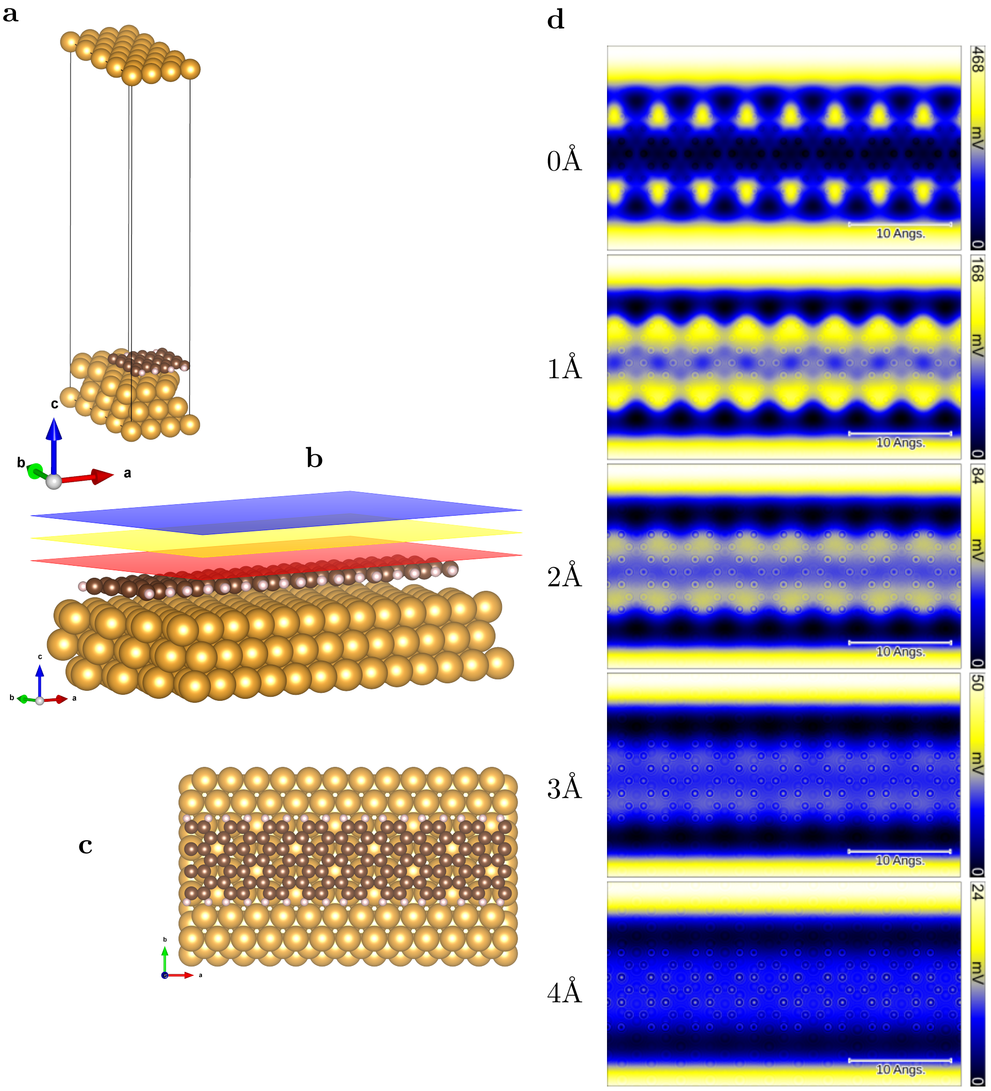


Figure 1: **a)** Orthorombic unit cell used in the calculations. **b)** The horizontal planes used to determine the LCPD maps for $s = 0$Å (red), $s = 2$Å (yellow) and $s = 4$Å (blue) are indicated above a $4 \times 1$ surface cell. **c)** Top view on the same cell and **d)** LCPD maps for the same cell and different values of $s$.
